# Supplementary material for: Grasping and Rolling In-plane Manipulation Using Deployable Tape spring Appendages
Source: arXiv:2412.00268 source file (2024-11-29)
Supplement: Supplementary file 1 [file supplementary_materials_GRIPtape_v1.pdf]

# Supplementary Materials for

## Grasping and Rolling In-plane Manipulation Using Deployable Tape-spring Appendages

Gengzhi He, Curtis Sparks, Nicholas Gravish

Corresponding author: ngravish@eng.ucsd.edu

**The PDF file includes:**

Materials and Methods
Figs. S1 to S6

**Other Supplementary Materials for this manuscript include the following:**

Movies S1 to S7

## Materials and Methods

Stiffness of the spring-like bending

The following section shows the relationship between the reaction force and the deformation of the spring-like bending.

$$\text{Bidirectional: } F = 0.00358x^3 + 0.00341x^2 + 0.66343x$$

$$\text{Unidirectional(convex): } F = 0.00144x^3 + 0.00266x^2 + 0.21346x$$

$$\text{Unidirectional(concave): } F = 0.00138x^3 + 0.00269x^2 + 0.20614x$$

Curve fit of the buckling force vs deployed length

$$F = 120.2069/(x - 8.2577) \quad \text{(Doublestack strong side)}$$

$$F = 88.4016/(x - 8.3434) \quad \text{(Bidirectional)}$$

$$F = 62.5938/(x - 8.7347) \quad \text{(Unidirectional)}$$

$$F = 22.0815/(x - 2.5518) \quad \text{(Doublectack weak side)}$$

CAD: Layout

The fabrication setup (Fig. S1A) mirrors the model discussed in Mechanism design and workspace. The layout includes 2 extruders positioned at the far left and far right of an acrylic base of size 450mm*200mm, directly controlling the supporting section of the appendages. Additionally, 2 extruders are managed by a rack and pinion mechanism located on a track in the middle. The angular control beams is linked to motors fixed directly on the base. In this design, there are 7 DYNAMIXELs employed, consisting of 5 XL430-W250-T units with a maximum stall torque of 1.5 Nm, and 2 XM540-W270-T units capable of delivering a stall torque of 10.60 Nm. The latter are utilized in constructing the angular control units, where substantial torque is necessary.

CAD: Width control

Shown in (Fig. S1B), the linear motion of the rack and pinion mechanism is constrained by two 8mm diameter metal rods that serves as the guiding track. The pinion with the radius of 14mm is driven by a DYNAMIXEL XL430-W250-T motor mounted below the base. Supported by 3 linear bearings each extruder on the track can travel on the linear track smoothly. Notably, the center of extruders (the contact point of rollers) is symmetrically placed around the pinion's rotational axis, meaning a line defined by two centers of extruder does travel though the rotational axis but is not in parallel with the rack (i.e., the parameter b is different for the two sets of appendages) to decrease the minimum gap between the extruders and enlarge the range of size of objects that GRIP-tape can handle. For the same reason, the triangular shape is adopted in designing the extruders on the racks.

CAD: Extruder

The extruder operates through a DYNAMIXEL XL430-W250-T motor, bifurcated into active and passive segments. Each segment features a roller on a shaft supported by $5\text{mm} * 10\text{mm} * 4\text{mm}$ bearings. They are fastened by four M3 screws, maintaining pressure on the rollers and facilitating friction adjustment as the screws' tightness regulates the roller-tape friction. The active roller is covered with sandpaper for increased traction. The extruder includes entrance and exit guides shaped to accommodate tape deformation to provide even support along the tape as they transform from soft to rigid. These guides play a crucial role in preventing the emergence of undesired bends caused by potential deformations in the tape due to its softness

when compressed between the two rollers and subjected to external forces. Fig. S1D provides a comparison between scenarios with and without guide support.

CAD: Angular control

The angular control unit (Fig. S1E) is responsible for adjusting $\theta_4$ , the largest affector on the direction appendages points. On the tip of the angular control link installs a guiding ring 115mm away from the motor axis that help holding the tape. The rotation axis of the guiding ring is intentionally offset from the beam to decrease potential collisions between the beam and the tape during movement of the beam. Additionally, an "X" shaped structure is integrated to stabilize the uprightness of the guiding ring, ensuring the tape's upright position in section view and further enhancing the overall gripping performance.

Inverse kinematics

In the following section we derive the inverse kinematics of an individual appendage. The inverse kinematics specifies a goal position of the appendage (x, y), and returns the required tape lengths and angles that place the center of the tape at that location. Fig. S2 illustrates the relevant geometry of the inverse kinematics.

the initial step involves determining the hypotenuses $L_1^*$ and $L_2^*$. The former can be computed as the square root of $x^2 + y^2$, while the latter is represented by the square root of $(a - x)^2 + (y + b)^2$.

Knowing $L_2^*$, and $r$, the right triangle (marked in red) is fully defined. The same applies to the other right triangle with $L_1^*$ as its adjacent.

It leads to the lengths of $L_1$, $L_2$, and angles $\theta_{12}$, $\theta_{22}$. The length of $L_3$ is defined as $(\theta_{31} + \theta_{32})r$.

While $\theta_{31} = \theta_{11} + \theta_{12}$ because of the 2 right angles in the blue quadrangle, similarly, $\theta_{32} = (\pi - \theta_{21}) + \theta_{22}$. $\theta_{11}$ and $\theta_{21}$ can be easily derived from another 2 right triangles (1 of them is marked in green) as $\theta_{11} = \tan^{-1}(y/x)$, $\theta_{21} = -\tan^{-1}((y + b)/(a - x))$.

For now, the only unknown is $\theta_4$, which equals to $(\theta_{11} + \theta_{12}) - \theta_5$, $\theta_5$ can be derived using the relation of the opposite $f$ and hypotenuse $L_4$. Where $f$ is adjacent of another triangle, it is calculated by $f = e\sin(\theta_f)$, and $\theta_f$ has a simple relationship with $\theta_{11}, \theta_{12}, and\ \theta_c$.

Calculate $L_1$ :

$$L_1^* = \sqrt{(x^2 + y^2)}$$
$$\theta_{11} = \tan^{-1}(y/x)$$
$$\theta_{12} = \sin^{-1}(r/L_1^*)$$
$$L_1 = L_1^*\cos(\theta_{12})$$

Calculate $L_2$ :

$$L_2^* = \sqrt{((a - x)^2 + (y + b)^2)}$$
$$\theta_{21} = -\tan^{-1}((y + b)/(a - x))$$
$$\theta_{22} = \sin^{-1}(r/L_2^*)$$
$$L_2 = L_2^*\cos(\theta_{22})$$

Calculate $L_3$ :

$$\theta_{31} = \theta_{11} + \theta_{12}$$
$$\theta_{32} = (\pi - \theta_{21}) + \theta_{22}$$

$$\theta_3 = \theta_{31} + \theta_{32}$$
$$L_3 = \theta_3 r$$

Calculate $\theta_4$ :

$$\theta_c = \tan^{-1}(c/d)$$
$$\theta_f = \pi - \theta_c - (\theta_{11} + \theta_{12})$$
$$e = \sqrt{(d^2 + c^2)}$$
$$\theta_5 = \sin^{-1}(e\sin(\theta_f)/L_4)$$
$$\theta_4 = (\theta_{11} + \theta_{12}) - \theta_5$$

Forward kinematics

For the forward kinematics, it outputs the coordinate of the center of the arc $(x, y)$ given $a$, $b$, $c$, $d$, $r$, $\theta_4$, $L_4$ and the total length $L$. We used $\theta_4$ to derive $\theta_1$:

$$\theta_1 = \tan^{-1}((L_4\sin(\theta_4) + c)/(L_4\cos(\theta_4) - d))$$

$L_1$, $L_2$, and $\theta_2$ can be derived by solving 3 nonlinear equations:

$$L = (L_1 + L_2 + r(\theta_1 - \theta_2 + \pi))$$
$$L_1\sin(\theta_1) + r\sin(\theta_1 - \pi/2) = (L_2\sin(\theta_2) + r\sin(\theta_2 + \pi/2) + b)$$
$$L_1\cos(\theta_1) + r\cos(\theta_1 - \pi/2) = (L_2\cos(\theta_2) + r\cos(\theta_2 + \pi/2) + a)$$

The coordinate of the center of the arc is:

$$x = L_1\cos(\theta_1) + r\cos(\theta_1 - \pi/2)$$
$$y = L_1\sin(\theta_1) + r\sin(\theta_1 - \pi/2)$$

Programming: Basic functions of single appendage

The control of GRIP-tape primarily relies on MATLAB, incorporating the DYNAMIXEL Protocol 2.0. This protocol enables the assignment of goal positions and velocities to specific addresses, facilitating the manipulation of the gripper's movement. Additionally, it allows for the report of present positions, aiding in determining the current configuration of the appendages through forward kinematics.

GRIP-tape is actuated by 7 DYNAMIXEL motors in extended position mode. Desired position can be reached with code provided by the manufacturer with assigning of position and velocity. Due to the built-in PID controller of DYNAMIXEL motors, no extra control of the position of motors is required.

Programming: Appendage transformation

Assuming the width control parameter a is known, the transformation of moving the center of the arc on the tip of the appendage to target location $(x^*, y^*)$ was conducted by steps:

**Step 0**: Set $\theta_{4i}$ to be 0, measure and input the initial $L_{1i}$, $L_{2i}$, $L_{0i}$. Record the states of both extruders and mark it as the initial state $E_{1i}$ and $E_{2i}$.

**Step 1**: Input the target coordinate $(x^*, y^*)$ of the center of the tip of the appendage and solve the inverse kinematics with known parameter a to find new target $L_1^*$, $L_2^*$, $L^*$ and $\theta_4^*$.

**Step 2**: Read the current state $E_1$ and $E_2$, current $L = L_i + (E_1 - E_{1i}) + (E_2 - E_{2i})$ and $\theta_4$. The configuration of the appendage including the current length of $L_1$, $L_2$ can be derived.

**Step 3**: There are 3 modes for appendage transformation: *Tip remain mode*: This mode ensures the object remains at a consistent relative distance in relation to the tip, particularly advantageous when the contacting point on the tape is close to the tip (Fig. S3A). Throughout the transformation, both extruders function independently, each extending by the lengths of $\delta E_1 =$

$\delta L - \delta E_2 = (L^* - L) - \delta E_2$ and $\delta E_2 = \delta L_2 \ = L_2^* - L_2$. As the contact surface (known as $L_2$) is the primary contact surface for the objects, in this mode what we want to ensure is $\delta E_2 = \delta L_2$ to make the point of tangency between link $L_2$ and arc $L_3$ on the physical tape keeps to be the point of tangency. Since the length of the curve $L_3$ varies during the transformation of the appendage, to make up the influence of $\delta L_3$, the computation of $\delta E_1$ relies on $\delta E_2$ and the difference between the target and current overall length $\delta L$.

*Outer only mode*: In this mode, the transformation is conducted with only functioning the extruder that directly controls the otter half of the appendage. It allows the appendages adjusting their length while keeping an object in grip stays in the global coordinate. Since the contacting surface is stalled, the axial movement is prohibited, to fulfill the task, the assigned coordinate must land on a certain line parallel to L_2 to avoid movements of the object in the angular direction (Fig. S3B).

*Inner only mode*: converse to the outer only mode, the inner only mode only drives the extruders that's on the track.

DYNAMIXELS stop after reaching the target positions controlled by the in-built PID controller.

**Step 4**: If new location is assigned, return to Step1

Rotation of appendages

Rotation of tape is conducted by extruding and retracting on 2 sides at the same speed. i.e., $\delta E_1 = -\delta E_2$. Since the overall length $L$, angle $\theta_4$, and width control parameter a are not changing, the shape of the appendage also remains the same.

Programming: Gripping objects

By inputting the coordinate $X_{obj} = (x, y)$ and the size of the object, in order to make the contact section of the appendages in parallel when gripping the object, so that the gripping force on each side are in exact countering directions to decrease the chance of slipping. The program adjusts the distance between the center of two inner extruders to $d'$ (Fig. S4) using the rack and pinion mechanism.

Programming: Translation of objects

The translation of objects involves both gripping and appendage transformation. Typically, it engages all 7 DYNAMIXEL motors. Upon receiving the object's target location, the program computes 2 sets of waypoints, each for one of the appendages along the trajectory from the current location to the target location, employing a similar approach described in the gripping process. Throughout the translation, the width is continuously adjusted to sustain the parallel configuration. During translation, a notable issue arises when assigning a constant velocity to all DYNAMIXEL motors between waypoints. This method does not result in a linear forward kinematics, meaning $(x, y)$ do not have linear relationship with any input, causing the actual trajectory of the arc's center to deviate from a straight line. Consequently, when holding an object, inconsistencies in the gripping force occur during translation, potentially leading mid-way drops. Presently, the solution involves setting closer waypoints to create a locally linear trajectory, aiming to mitigate this issue.

Programming: Rotation and conveying of objects

These functions exclusively involve rotating the appendages. Object rotation occurs when both appendages rotate in the same direction and at equal speeds, causing the contact sections to move in opposing directions. The resulting friction forces counterbalance each other, yielding solely a rotational moment on the object, thereby initiating its rotation. Conveying, on the other hand, arises when the appendages rotate in opposite directions. It's crucial to highlight that conveying is feasible only when the gap between the contact sections of the appendages remains unchanged, i.e., the parallel alignment. Furthermore, within this setup, the rotational and conveying actions can be mixed by applying different rotation speeds to each appendage. For instance, by halting the rotation of one appendage, it works solely as a supportive track, enabling the object to roll in a specific direction on it.

<u>Programming: App design</u>

Utilizing MATLAB functions, an app was created using the MATLAB app designer (Fig. S5). The app includes two switches for starting up the gripper. One is responsible for loading the library into MATLAB, while the other activates the motor power. Usually, before each operation, pressing the “set initial” button reads the current positions of most motors and sets them as the initial states. For the angular control units, this button also drives the angular control links to desired initial angles. The “to initial” button will drive the appendages back to their initial state within a given amount of time.

After the main switch turns on, the value of the x slider and the y slider will be assigned as the target location, and the two appendages will start to translate to this position the way discussed in Programming: Appendage transformation with a mode chosen in the “Mode” block. A while loop will keep checking the target location, and reading the current states of each motor. By changing the x and y values on the sliders, it will assign new target location to the appendages. Slider “w” and “g” are responsible for adjusting the gap between the two appendages at the base and the gripping force. The plot on the upper right will keep updating with the predicted lay out of the appendages after each input of a different target location. The “STOP” switch is an emergency stop that stops any ongoing task when it is on.

The “Auto” switch initiates the automatic object detection, measurement, and gripping process. “F base”, “F tip”, and “F obj” display the force readings at the base, the predicted force at the appendages' tip, and the anticipated force on the object.

<u>Programming: Control with game pad</u>

The integration of game-pad control within the app enables object manipulation in location via Logitech F310's right joystick, adjusting the target location within a maximum of 10mm increment per loop cycle. The left joystick's x-axis regulates the parameter “w” (gap), while the triggers (RT tighten & LT loosen) manage the “g” (gripping force). Appendage rotation is linked to the shoulders (RB & LB) for different directions. Pressing either shoulder initiates object rotation, while button “A” reverses the rotation direction of one appendage, conveying the object inward or outward based when the respective shoulder is pressed.

<u>Calculation of the gripping force</u>

$$F_1' = F_{read}/\cos(\theta_1 - \theta_4)$$

$$F_1 = (F_1{}' * L_1{}' + \tau_1)/L_1 \qquad \text{(Balance of moments on } L_1\text{)}$$

$$F_2 = F_1$$

$$F_2' = (F_2 * L_2 + \tau_2)/L_2{}' \qquad \text{(Balance of moments on } L_2\text{)}$$

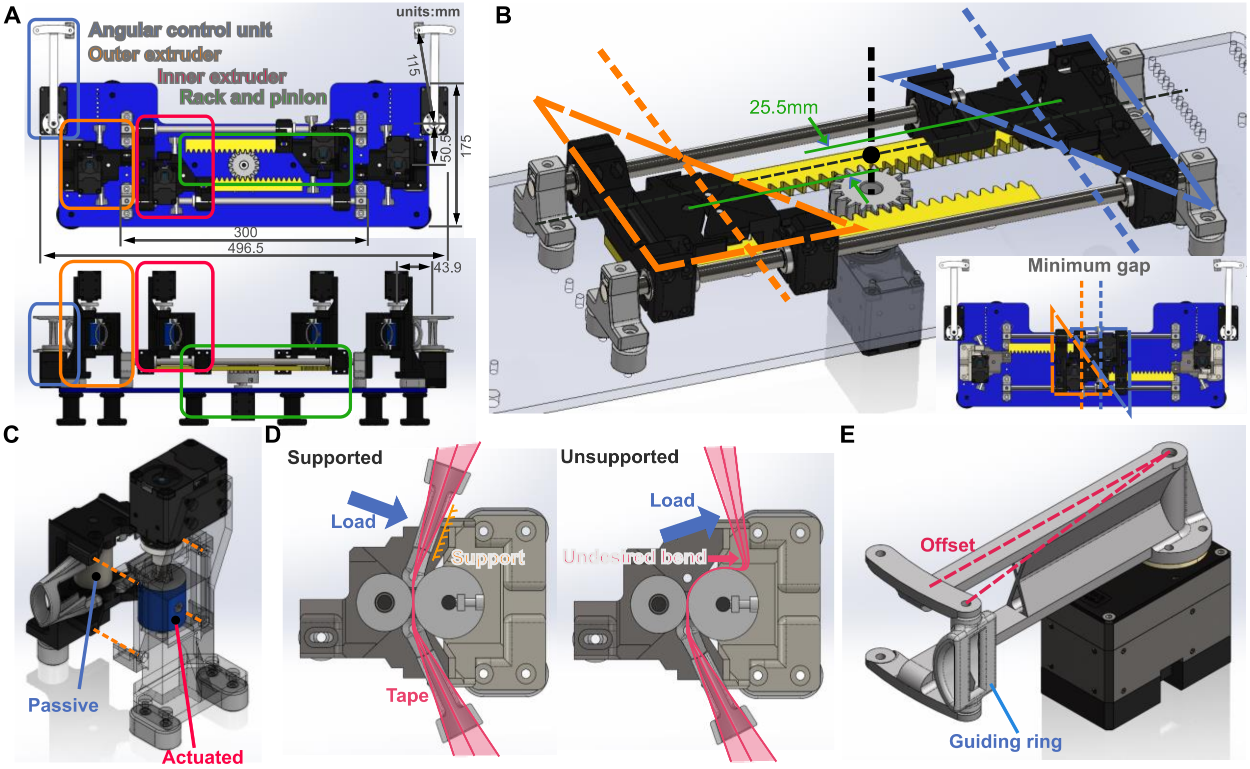


**Fig. S1.**

**CAD of the GRIP-tape.** (**A**) Layout of the CAD. (**B**) The width control unit. (**C**) The extruder. (**D**) The supporting guide. (**E**) The angular control unit.

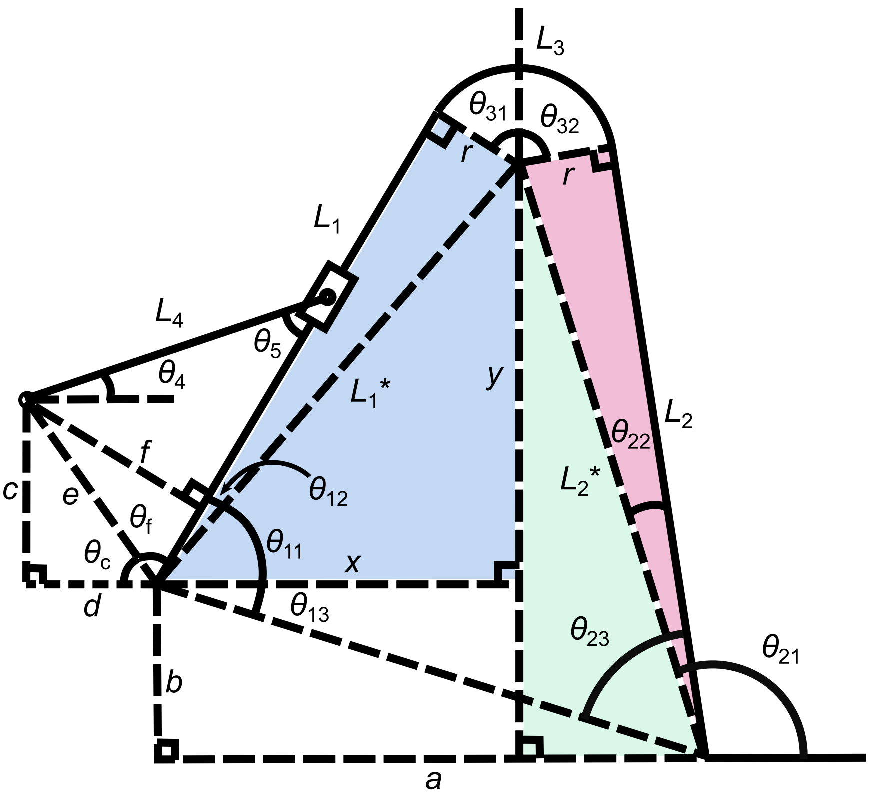


**Fig. S2.**
**Illustration for the inverse kinematics.**

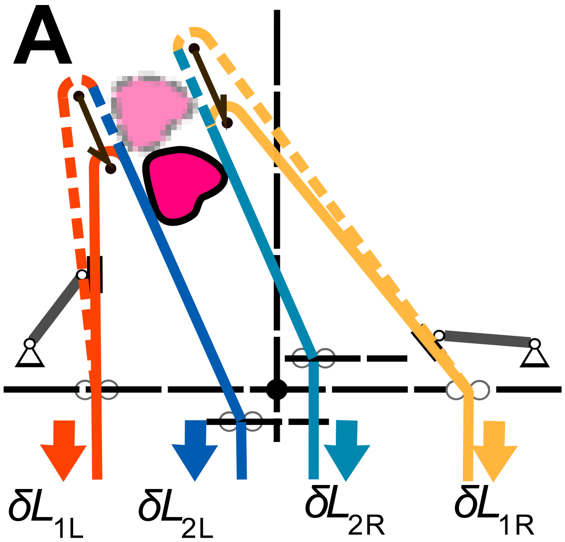


**Fig. S3.**

**Different transformation modes of the appendage.** (**A**) Mode: tip remain. (**B**) Mode: outer only.

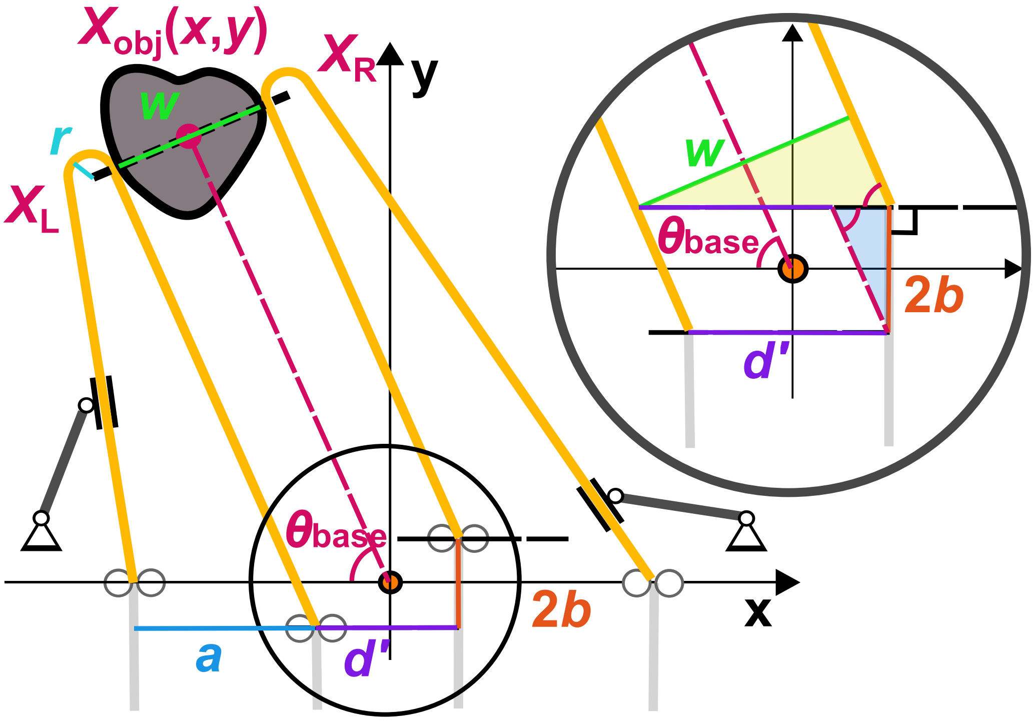


**Fig. S4.**

**Width adjustment on the base during gripping and translation.**

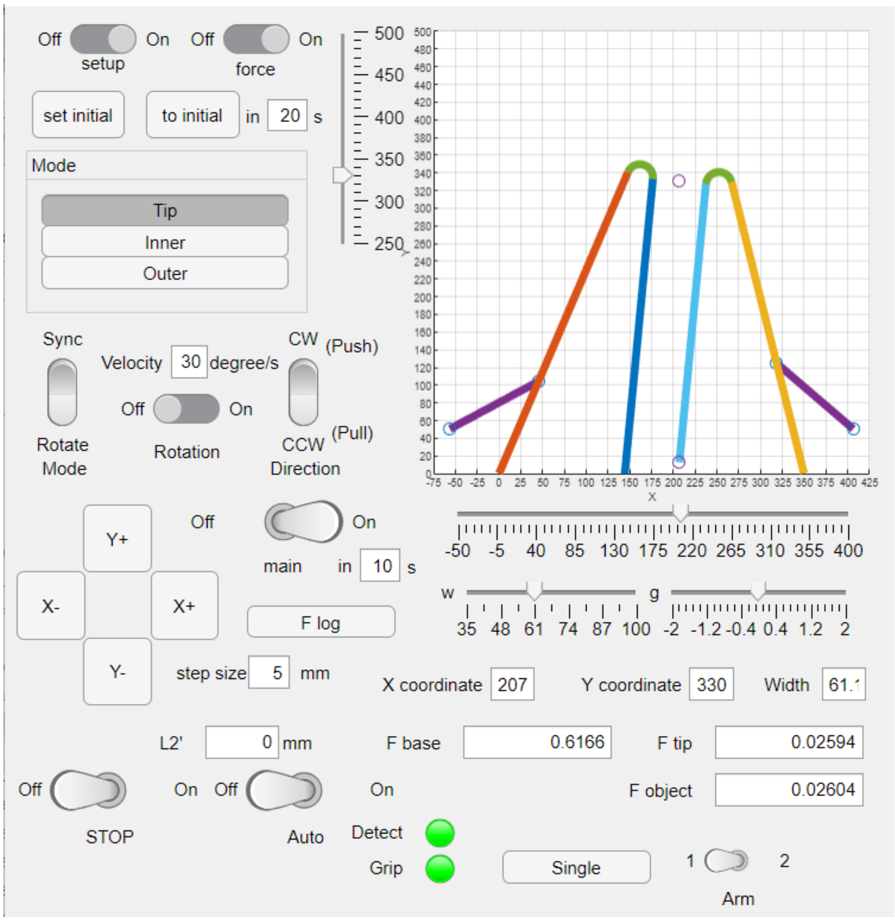


**Fig. S5.**
**App design.**

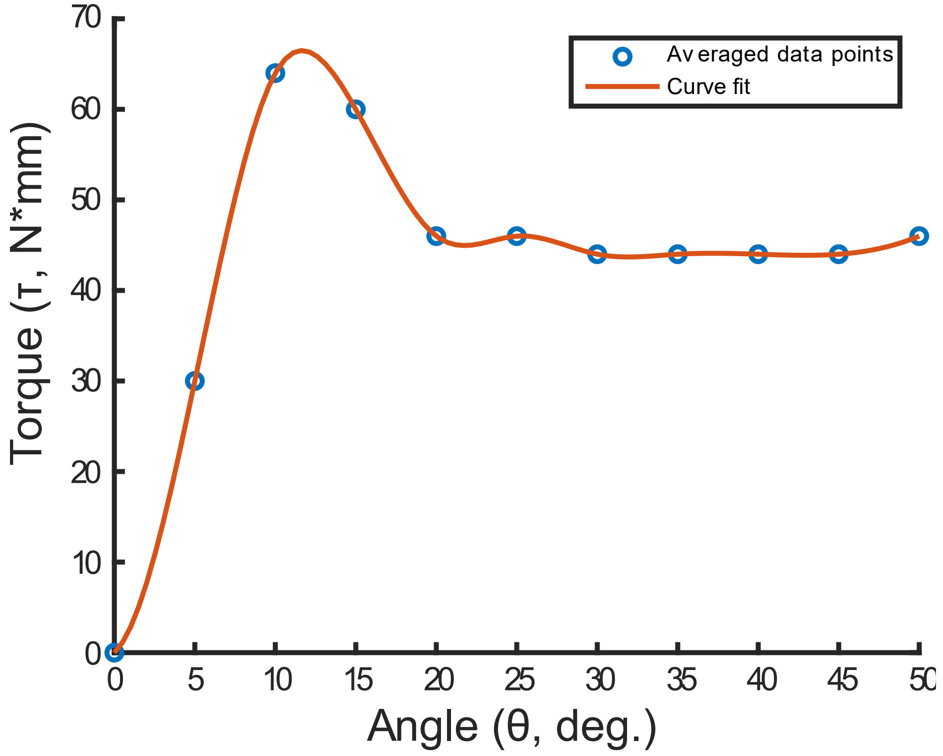


**Fig. S7.**
**Data points and curve fit of the internal torque of bidirectional tape.**

**Movie S1.**
Properties of tape spring.

**Movie S2.**
Bidirectional tape - extension and spooling.

**Movie S3.**
Demonstration of basic abilities.

**Movie S4.**
Applications.

**Movie S5.**
Features of the tape spring appendages.

**Movie S6.**
Automatic gripping.

**Movie S7.**
Feedback Control.
